# Supplementary material for: MiniOS: an instructional platform for teaching operating systems labs
Source: arXiv:1811.09792 source file (2018-12-01)
Supplement: Supplementary file 1 [file appendix.pdf]

## 9.3 Running apps on MiniOS

Running apps is a straightforward task, but it requires some understanding of how the machine executes instructions and how the compiler generates this code. As usual, let us demonstrate with an example. Say, we already have MiniOS (up to the HAL) living in program memory. Now what? How do we execute an application? Well, first we need an application. Moreover, it must be a stand-alone application that is not compiled with the HAL. Listing 9.1 shows a simple stand-alone application written in assembly that uses the drivers pio.s writen for the IO chapter (Section 4.3) to drive LED0 on.

```
#define OUTPUT_DIR  0
#define LEVEL_LOW   0

void main(void){
   pioc_init();
   pioc_dir_set( OUTPUT_DIR, 23 );
   pioc_level_set( LEVEL_LOW, 23 );
}
```

Listing 9.1: Sample App

Because its a stand-alone application, creating an Atmel Studio project to compile it is different from what the reader has done before. The exact steps are demonstrated in Executing Applications—How to create a stand-alone C project.

Now we have an application. What is next? We want this application to run from RAM. *How* do we tell that an application must run RAM? More importantly, *who* do we tell that to? The *who* is the linker. The linker is the one responsible for address resolution (Section 3.4). Therefore, the *how* is the linker script (Section 3.5). The linker script for our sample stand-alone C project is split in two files, *sam4s_flash.ld*, and *sam4sd32c_flash.ld*. (For some reason Atmel decided to split it, it makes no difference.) Part of the linker script structure is shown in Listing 9.2.

```
MEMORY{
  rom (rx)  : ORIGIN = 0x00400000, LENGTH = 0x00200000
  ram (rwx) : ORIGIN = 0x20000000, LENGTH = 0x00028000
}
SECTIONS{
    .text : {
```

# Chapter 10

# System Calls

> All problems in computer science can be solved by another level of indirection
>
> David J. Wheeler

Thus far there is one problem related to how system and applications co-exist. Namely, **applications have full access to OS code and data, and are thus capable of manipulating them, whether intentionally or not.** When modification is intentional the problem falls under security, and the idea is to prevent malicious code from messing with the system, e.g., crashing it or leaking sensible information[1]. On the contrary, when it is not intentional, it is a matter of fault tolerance, and the idea is to prevent an application bug to crash the entire system and cause unwanted side effects[2].

In either case, granting applications arbitrary access to the kernel is a bad idea. To show this more concretely, lets look at an example. (Before continuing make sure to check the solution to the previous lab[3])

Consider the code in Listing 10.1. This piece of code executes OS code and modifies OS data, as shown in Demo—messing with the system.

[1] See for instance, Android Bug Exploit (there's a video in it)

[2] See for example, Toyota's unintended acceleration case

[3] For a demo of the solution see this. To set up PuTTY see here

# A.4 On-board and expansion boards examples

This section includes peripheral part of the SAM4S board, and its expansion boards.

## A.4.1 Buttons

Unlike other GPIO-based devices, mechanical buttons are peculiar: when pressed, they bounce. We like to think that when a button is pressed it will change the IO line's state and when the button is released its state will go back. Something like this:

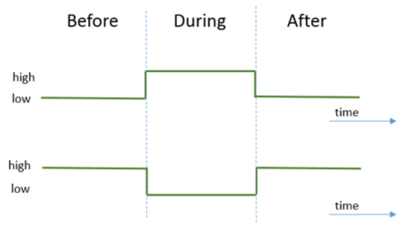


Figure A.2: Button Ideal

The physical world is never that ideal, however. When a mechanical button is pressed it bounces, therefore generating a train of pulses instead of just one.

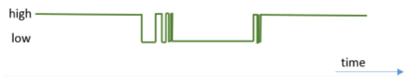


Figure A.3: Button real

This is then interpreted as the button being pushed several times. The ATSAM4SDC32 has hardware support for de-bouncing, which allows to filter pulses which duration is less than a specified threshold. This will not eliminate all the glitches, but it will make it much better; so expect a few of them when you press buttons. Another way is to do it by software, but this requires intervention of the CPU. The idea is the same, whenever a change in state is detected in an IO line, check the IO line again a few milliseconds later; if the state is the same then the button
